# Supplementary material for: An Integrated Approach for Energy Efficient Handover and Key Distribution Protocol for Secure NC-enabled Small Cells
Source: arXiv:2205.08641 source file (2022-05-17)
Supplement: Supplementary file 1 [file appendix.tex]

\newlist{abbrv}{itemize}{1}
\setlist[abbrv,1]{label=labelwidth=1in,align=parleft, left = 1pt..7em}
\addcontentsline{toc}{chapter}{List of Abbreviations}
\chapter*{List of Abbreviations}
\chaptermark{List of Abbreviations}
\begin{abbrv}
\item[5G] Fifth Generation of cellular networks.
\item[AMF] Access and Mobility Management Function.
\item[B5G] Fifth Generation and Beyond.
\item[BFT] Byzantine Fault Tolerance.
\item[BS] Base Station.
\item[BSH] Blockchain-based Security and HO.
\item[D2D] Device to Device.
\item[DL] Downlink.
\item[DLRS] Downlink Refernce Signal.
\item[eNB] eNodeB.
\item[HMAC] Homomorphic MAC.
\item[HO] Hand Over.
\item[ISD] Inter Site Distance.
\item[KDC] Key Distribution Center.
\item[LTE] Long Term Evolution.
\item[MAC] Message Authentication Codes.
\item[MME] Mobility Management Entity.
\item[NC] Network Coding.
\item[NR] New Radio.
\item[RACH] Random Access Channel.
\item[RLNC] Random Linear Network Coding.
\item[RRM] Radio Resource Management.
\item[s-BS] Serving Base Station.
\item[SDG] Serving Data Gateway.
\item[t-BS] Target Base Station.
\item[UDG] User Data Gateway.
\item[UE] User Equipment.
\item[UL-HO] ULRS-based HO.
\item[ULRS] Uplink Reference Signal. 
\item[UL-RSRP] UL-RS Received Power.
\item[UL-TTT] UL Time to Trigger.
\item[UPF] User Plane Function.
\end{abbrv}
